# Supplementary material for: Questioning the Questions: Sustaining Self-Evolution in Reasoning Models
Source: arXiv:2610.04299 source file (2026-10-06)
Supplement: Supplementary file 1 [file prompt_setup.tex]

% Load in the preamble, before \begin{document}. Safe to input more than once.
\ifdefined\captionof\else
  \RequirePackage{capt-of}
\fi
\RequirePackage{tcolorbox}
\tcbuselibrary{breakable,skins}

\ifdefined\paperprompt\else
% Numbered prompt captions; reset within each section (e.g., Prompt A.1).
\newtcolorbox[auto counter,number within=section]{paperprompt}[2][]{
  enhanced,
  breakable,
  colback=black!2,
  colframe=black!25,
  colbacktitle=black!5,
  coltitle=black,
  boxrule=0.4pt,
  arc=1mm,
  left=7pt,right=7pt,top=6pt,bottom=6pt,
  before skip=8pt,after skip=8pt,
  fontupper=\normalfont\small,
  fonttitle=\normalfont\small\bfseries,
  title={Prompt~\thetcbcounter: #2},
  title after break={Prompt~\thetcbcounter: #2 (continued)},
  #1
}
\fi
